# Supplementary material for: Asymptotic formulae for flow in superhydrophobic channels with longitudinal ridges and protruding menisci
Source: arXiv:1712.03104 ancillary file (2018-01-29)
Supplement: Supplementary file 1 [file Supplementary_materials.pdf]

Supplementary material for

# Asymptotic formulae for flow in superhydrophobic channels with longitudinal ridges and protruding menisci

Toby L. Kirk

*Department of Mathematics, Imperial College London, London SW7 2AZ, UK*

## 1 Solution of the inner problem for $\delta \ll 1$

In this section of supplementary material, we derive the solution to the problem for $\widehat{W}$ given by (3.5)-(3.8) of the paper in the limit $\delta \ll 1$.

First, we state the problem for the complex potential $\hat{h}(z)$ such that $\widehat{W} = \mathrm{Im}\{\hat{h}(z)\}$, $z = X + \mathrm{i}Y$. The no-slip condition on the ridges, and the far-field condition (3.8) can then be written as

$$\mathrm{Im}\left\{\hat{h}(z)\right\} = 0, \qquad \text{on } Y = 0,\ X \notin [-\delta, \delta] \tag{1}$$

$$\hat{h}(z) \sim z + \mathrm{i}\hat{\lambda}(\epsilon), \qquad \text{as } z \to \infty. \tag{2}$$

Periodicity of $\widehat{W}$ implies that $\hat{h}(z)$ must have quasi-periodicity, i.e, for each $n \in \mathbb{Z}$, $\hat{h}(z+2n) = \hat{h}(z) + k$ for some $k \in \mathbb{R}$. If $s$ is the arclength along the meniscus, measured from $X = -\delta$ in the direction of increasing $X$, the condition on the meniscus can be written, using the Cauchy–Riemann relations,

$$\frac{\partial}{\partial s}\mathrm{Re}\left\{\hat{h}(z)\right\} = [1 + \epsilon\hat{\lambda}(\epsilon)]\frac{2\epsilon Y}{(1+Y'^2)^{1/2}}, \qquad \text{on the meniscus } S. \tag{3}$$

Integrating with respect to arclength and substituting $\mathrm{d}s = (1 + Y'^2)^{1/2}\mathrm{d}X$ gives, up to a real additive constant:

$$\mathrm{Re}\left\{\hat{h}(z)\right\} = [1 + \epsilon\hat{\lambda}(\epsilon)]\int 2\epsilon Y(X)\mathrm{d}X, \qquad \text{on the meniscus } S. \tag{4}$$

The meniscus shape is denoted by $|z - C| = R$, where $C$ is the centre of the circle (which is pure imaginary) and $R$ the radius, given by

$$R = \frac{\delta}{\sin\theta}, \qquad C = -\mathrm{i}\delta\cot\theta. \tag{5}$$

Therefore, on the meniscus $\bar{z} = \bar{C} + R^2/(z - C)$, and consequently

$$Y(X) = \frac{1}{2\mathrm{i}}(z - \bar{z}) = \frac{1}{2\mathrm{i}}\left(z - \bar{C} - \frac{R^2}{z - C}\right), \quad \mathrm{d}X = \frac{1}{2}(\mathrm{d}z + \overline{\mathrm{d}z}) = \frac{1}{2}\left(1 - \frac{R^2}{(z - C)^2}\right)\mathrm{d}z. \tag{6}$$

Using the above expressions for $Y(X)$ and $\mathrm{d}X$ in terms of $z$, the integral (4) over the meniscus can be evaluated, giving

$$\begin{aligned}\mathrm{Re}\left\{\hat{h}(z)\right\} = \chi(z) =& [1 + \epsilon\hat{\lambda}(\epsilon)]\frac{\epsilon}{2\mathrm{i}}\left[\frac{1}{2}(z - C)^2 + 2C(z - C) - 2R^2\log\left(\frac{z - C}{R}\right)\right. \\ &\left. + \frac{2CR^2}{z - C} - \frac{R^4}{2(z - C)^2}\right], \qquad \text{on the meniscus,}\end{aligned} \tag{7}$$

up to an arbitrary real constant.

## 1.1 Complex potential for a single meniscus or groove

The first step in finding a solution to the above problem in the limit $\delta \ll 1$, is to consider the non-periodic case of a single meniscus or groove occupying $X \in [-\delta, \delta]$. If we denote the corresponding complex potential by $\hat{h}_s(z)$, then the solution we seek is analytic in the upper half plane external to the meniscus, satisfying conditions (1), (7), and $\hat{h}_s(z) \sim z$ as $z \to \infty$. We employ the conformal map (see Crowdy [1])

$$z(\zeta) = \delta\frac{(1 - \zeta)^\alpha + (1 + \zeta)^\alpha}{(1 - \zeta)^\alpha - (1 + \zeta)^\alpha}, \qquad \alpha = \frac{2}{\pi}(\pi - \theta), \tag{8}$$

from the auxiliary $\zeta$ domain, $D_\zeta$, consisting of the upper half of the unit disk. The meniscus maps to the upper semi-circle $C^+ = \left\{\zeta = \mathrm{e}^{\mathrm{i}\phi} : 0 \leq \phi \leq \pi\right\}$, and the no-slip boundary to the real axis, $\zeta \in [-1, 1]$. The behaviour $\hat{h}_s(z) \sim z$ as $z \to \infty$ corresponds to $\hat{h}_s(z(\zeta)) \sim -\delta/(\alpha\zeta)$ as $\zeta \to 0$ in $D_\zeta$. We write the solution as $\hat{h}_s(z) = h_s(z) + \hat{H}(\zeta)$, where

$$h_s(z) = \frac{\delta}{\alpha}\left(\zeta(z) - \frac{1}{\zeta(z)}\right), \tag{9}$$

is the solution to the same problem as $\hat{h}_s(z)$ but with a no-shear stress condition on the meniscus, $\mathrm{Re}\{h_s(z)\} = 0$ [1]. Then $\hat{H}(\zeta)$ satisfies the same problem as $\hat{h}_s(z)$, but is now analytic as $\zeta \to 0$, and all of $D_\zeta$. Moreover, $\mathrm{Im}\{\hat{H}(\zeta)\} = 0$ for $\zeta = [-1, 1]$ means $\hat{H}(\zeta)$ is real on $\zeta \in [-1, 1]$ and the Schwarz Reflection Principle ([4] pp. 184) can be used to extend $\hat{H}(\zeta)$ analytically to the whole unit $\zeta$-disk, via $\hat{H}(\zeta) = \overline{\hat{H}(\bar{\zeta})}$. This relation gives a condition for $\hat{H}(\zeta)$ on the lower semi-circle $C^- = \left\{\zeta = \mathrm{e}^{\mathrm{i}\phi} : -\pi \leq \phi \leq 0\right\}$:

$$\mathrm{Re}\left\{\hat{H}(\zeta)\right\} = \mathrm{Re}\left\{\hat{H}(\bar{\zeta})\right\} = \mathrm{Re}\left\{\hat{H}(\zeta^{-1})\right\}, \qquad \text{for } \zeta \in C^-, \tag{10}$$

using $\bar{\zeta} = \zeta^{-1}$ on $C^-$. Therefore,

$$\mathrm{Re}\left\{\hat{H}(\zeta)\right\} = \begin{cases} \chi\left[z(\zeta)\right] & \text{for } \zeta \in C^+, \\ \chi\left[z(\zeta^{-1})\right] & \text{for } \zeta \in C^-. \end{cases} \tag{11}$$

As $\hat{H}(\zeta)$ is analytic in the unit disk with its real part specified on the boundary, the solution can be given by the Poisson integral formula ([4] pp. 17). The solution for $\hat{h}_s(z(\zeta)) = (\delta/\alpha)(\zeta - \zeta^{-1}) + \hat{H}(\zeta)$ is then

$$\begin{aligned} \hat{h}_s(z(\zeta)) =& \frac{\delta}{\alpha}\left(\zeta - \frac{1}{\zeta}\right) + \frac{1}{2\pi\mathrm{i}}\int_{C^+} \frac{\mathrm{d}\zeta'}{\zeta'}\frac{\zeta'+\zeta}{\zeta'-\zeta}\chi\left[z(\zeta)\right] \\ &+ \frac{1}{2\pi\mathrm{i}}\int_{C^-} \frac{\mathrm{d}\zeta'}{\zeta'}\frac{\zeta'+\zeta}{\zeta'-\zeta}\chi\left[z(\zeta^{-1})\right], \end{aligned} \tag{12}$$

with $\chi(z)$ given by (7). Of particular interest is an expression for $\mathrm{Im}\{\hat{h}_s(z)\}$ at the meniscus. For $z$ on the meniscus, $\zeta \in C^+$, we can write $\zeta = \mathrm{e}^{\mathrm{i}\phi}$, $\zeta' = \mathrm{e}^{\mathrm{i}\psi}$ and use the Plemelj formula to give

$$\mathrm{Im}\{\hat{h}_s(z)\} = \frac{2\delta}{\alpha}\sin\phi + [1+\epsilon\hat{\lambda}(\epsilon)]\frac{\epsilon\delta^2}{2\pi}⨍_{-\pi}^{\pi} \mathrm{d}\psi\, \cot\left(\frac{\phi-\psi}{2}\right)g(\psi), \tag{13}$$

where $g(\psi)$ is the even function

$$\begin{aligned} g(\psi) =& \csc^2\theta\,\mathrm{i}\log\left[\mathrm{i}\frac{\mathrm{e}^{\mathrm{i}\theta/2} + \mathrm{e}^{-\mathrm{i}\theta/2}\tan^{\alpha}(|\psi|/2)}{\mathrm{e}^{-\mathrm{i}\theta/2} + \mathrm{e}^{\mathrm{i}\theta/2}\tan^{\alpha}(|\psi|/2)}\right] \\ &+ \csc\theta\frac{[1-\tan^{2\alpha}(|\psi|/2)][\cos\theta + 2\cos 2\theta\tan^{\alpha}(|\psi|/2) + \cos\theta\tan^{2\alpha}(|\psi|/2)]}{[1+2\cos\theta\tan^{\alpha}(|\psi|/2) + \tan^{2\alpha}(|\psi|/2)]^2}. \end{aligned} \tag{14}$$

## 1.2 Exact formula for $\hat{\lambda}(\epsilon)$ using a reciprocal result

Using Green's second identity, a formula for the unknown $\hat{\lambda}(\epsilon)$ can be found by means of a reciprocity result due to Crowdy [2] that can account for any inhomogeneity in the condition on the meniscus. Let $V$ be the solution to the same problem as $\widehat{W}$ but with a homogeneous no-shear condition at the meniscus, $\mathbf{n}\cdot\nabla V = 0$ (alternatively, $V$ corresponds to $\widehat{W}$ with $\epsilon = 0$). If they have behaviours at infinity given by

$$\widehat{W} \sim Y + \hat{\lambda}(\epsilon), \qquad \text{as } Y \to \infty, \tag{15}$$

$$V \sim Y + \lambda, \qquad \text{as } Y \to \infty, \tag{16}$$

then the reciprocal result of [2] gives

$$\hat{\lambda}(\epsilon) = \lambda - \frac{1}{2}[1 + \epsilon\hat{\lambda}(\epsilon)] \int_S \frac{2\epsilon Y}{(1 + Y'^2)^{1/2}} V \,\mathrm{d}s. \tag{17}$$

Rearranging (17) to solve for $\hat{\lambda}(\epsilon)$, and using $\mathrm{d}s = (1 + Y'^2)^{1/2}\mathrm{d}X$, we find

$$\hat{\lambda}(\epsilon) = \frac{\lambda - \epsilon \int_S YV \,\mathrm{d}X}{1 + \epsilon^2 \int_S YV \,\mathrm{d}X}. \tag{18}$$

This is exact, and reduces to $\lambda$ when $\epsilon = 0$, as expected. We note that $V$ and $\lambda$ do not depend on $\epsilon$, only on $\delta$ and $\theta$.

If $V = \mathrm{Im}\{h(z)\}$, with successive approximations $h_0, h_1, \ldots$, in $\delta \ll 1$, then substitution into (18) gives corresponding approximations to $\hat{\lambda}(\epsilon)$.

## 1.3 Approximations to $\hat{\lambda}(\epsilon)$ for $\delta \ll 1$

Crowdy's first two approximations to $h(z)$ are given in our notation by

$$h_0(z) = h_s(z) + \lambda_0 \left[\frac{2}{\pi z} - \cot\left(\frac{\pi z}{2}\right)\right], \qquad \lambda_0 = \delta^2 \frac{3\pi^3 - 4\pi^2\theta + 2\pi\theta^2}{12(\pi - \theta)^2}, \tag{19}$$

$$h_1(z) = h_s(z) + \lambda_1 \left[\frac{2}{\pi z} - \cot\left(\frac{\pi z}{2}\right) + \frac{\pi}{6}(h_s(z) - z)\right], \quad \lambda_1 = \frac{\lambda_0}{1 - \frac{1}{6}\pi\lambda_0}, \tag{20}$$

where $h_s(z)$ is the solution of for a single shear-free meniscus, (9). If we work from (19), which is correct to $O(\delta^2)$, we see that $\int_S YV \,\mathrm{d}X \sim \int_S Y^2 \,\mathrm{d}X = O(\delta^3)$, which should be neglected in (18) at this level of approximation, giving $\hat{\lambda}_0(\epsilon) = \lambda_0$. However, this greatly decreases the accuracy of the $\epsilon$ expansion, as all $\epsilon$ dependence has dropped out. Therefore, we must work with a higher order approximation in $\delta$ to retain this integral term with confidence.

Approximation (20) is correct to $O(\delta^4)$, and if we substitute $V = \mathrm{Im}\left\{(1 + \frac{1}{6}\pi\lambda_1)h_s(z)\right\} + O\left(\delta^2\right)$ into (18) and use (6), we have

$$\hat{\lambda}_1(\epsilon) = \frac{\lambda_1 - \left(1 + \frac{1}{6}\lambda_1\pi\right)\epsilon J}{1 + \left(1 + \frac{1}{6}\lambda_1\pi\right)\epsilon^2 J}, \tag{21}$$

where

$$J = \int_S \mathrm{Im}\{h_s\}\, Y \mathrm{d}X \tag{22}$$

$$= \int_S \mathrm{Im}\left\{\frac{\delta}{\alpha}\left(\zeta(z) - \frac{1}{\zeta(z)}\right)\right\} \frac{1}{2\mathrm{i}}\left(z + C - \frac{R^2}{z - C}\right) \frac{1}{2}\left(1 - \frac{R^2}{(z - C)^2}\right) \mathrm{d}z. \tag{23}$$

The meniscus in the $\zeta$-plane is given by the unit semi-circle, $\left\{\zeta = \mathrm{e}^{\mathrm{i}\phi} : 0 \le \phi \le \pi\right\}$, so $\bar{\zeta} = 1/\zeta$ on the meniscus. Transforming the integration to the $\zeta$-plane via (8) and substituting $\zeta = \mathrm{e}^{\mathrm{i}\phi}$,

(23) simplifies to $J = \delta^3 I(\theta)$ where $I(\theta)$ is a function of $\theta$ only,

$$I(\theta) = 8\sin\theta \int_0^\pi \frac{\tan^{2\alpha}(\phi/2)[\cos\theta\tan^{2\alpha}(\phi/2) + 2\tan^\alpha(\phi/2) + \cos\theta]\,\mathrm{d}\phi}{[\tan^{2\alpha}(\phi/2) + 2\cos\theta\tan^\alpha(\phi/2) + 1]^3}. \tag{24}$$

One may notice that $\left(1 + \frac{1}{6}\lambda_1\pi\right)\epsilon J = \epsilon J + O(\delta^5)$, and the term $\frac{1}{6}\lambda_1\pi$ could be neglected in (21). But it can be kept with no effort, and has a significant effect on accuracy when $\theta$ is large. Indeed, $\hat{\lambda}_1(\epsilon)$ in the form (21) appears naturally from the construction of the complex potential.

## 1.4 Expression for the complex potential

Here we justify the approximation given by (4.2) in the paper to the complex potential $\hat{h}(z)$ that is the solution to (1)-(7). We will only show that $\hat{h}_1(z)$ approximately satisfies the problem, as the argument is similar for $\hat{h}_0(z)$.

The approximation restated here is

$$\hat{h}_1(z) = \hat{h}_s(z) + \hat{\lambda}_1\left[\frac{2}{\pi z} - \cot\left(\frac{\pi z}{2}\right) + \frac{\pi}{6}(h_s(z) - z)\right], \tag{25}$$

where $\hat{h}_s(z)$ and $h_s(z)$ are (12) and (9), and assume $\hat{\lambda}_1$ is not yet known. Potential (25) is analytic in the period window, as the pole at $z = 0$ is removable, and $\hat{\lambda}_1$ is chosen to ensure that the $O(1/z)$ term of $\hat{h}_s(z)$ as $z \to \infty$ is removed, resulting in $\hat{h}_1(z) \sim z + \mathrm{i}\hat{\lambda}_1 + O(1/z^3)$. For this, the behaviours of $\hat{h}_s(z)$ and $h_s(z)$ as $z \to \infty$ are needed. If

$$\hat{h}_s(z) \sim z + \frac{\hat{\Delta}}{z} + O\left(\frac{1}{z^3}\right), \qquad z \to \infty, \tag{26}$$

$$h_s(z) \sim z + \frac{\Delta}{z} + O\left(\frac{1}{z^3}\right), \qquad z \to \infty, \tag{27}$$

then

$$\hat{\Delta} + \frac{2\hat{\lambda}_1}{\pi} + \frac{\pi\hat{\lambda}_1}{6}\Delta = 0. \tag{28}$$

From (8), (9), we know $\Delta = -\delta^2(2/\alpha^2 + 1)/3$, and $\hat{\Delta}$ can be found from expanding the integral formula (12). Using (8), $\hat{\Delta}$ can be found from the series as $\zeta \to 0$ in the $\zeta$-plane via

$$\hat{h}_s(z(\zeta)) = -\frac{\delta}{\alpha\zeta} - \left[\frac{(\alpha^2 - 1)\delta}{3\alpha} + \frac{\alpha}{\delta}\hat{\Delta}\right]\zeta + O(\zeta^3), \qquad \zeta \to 0. \tag{29}$$

Expanding the Poisson kernal $(\zeta' + \zeta)/(\zeta' - \zeta) = 1 + 2\zeta/\zeta' + \cdots$ and then substituting $\zeta \mapsto 1/\zeta$ in the integral over $C^-$ and performing integration by parts, formula (12) can be shown after some algebra to have the expansion

$$\hat{h}_s(z(\zeta)) = -\frac{\delta}{\alpha\zeta} + \left[\frac{\delta}{\alpha} - 2\epsilon(1 + \epsilon\hat{\lambda}_1)\frac{\alpha}{\pi\delta}J\right]\zeta + O(\zeta^3), \qquad \zeta \to 0. \tag{30}$$

Equating coefficients of $\zeta$ determines $\hat{\Delta}$ to be

$$\hat{\Delta} = \Delta + 2\epsilon(1 + \epsilon\hat{\lambda}_1)\frac{1}{\pi}J, \tag{31}$$

and on substituting into (28) gives

$$\hat{\lambda}_1 = \frac{-\frac{\pi}{2}\Delta - \epsilon J}{1 + \frac{\pi^2}{12}\Delta + \epsilon J}.$$

But $\lambda_1$ for the homogeneous case $\epsilon = 0$ is given by $\lambda_1 = -\frac{\pi}{2}\Delta/(1 + \frac{\pi^2}{12}\Delta)$, and eliminating $\Delta$ in the above results in exactly the expression (21), found by the reciprocal result.

Finally it remains to show (25) satisfies conditions (1) and (7) to $O(\delta^4)$. As $\hat{h}_s(z)$, $h_s(z)$ and the remaining terms in (25) are real for $z \in \mathbb{R}\backslash[-\delta, \delta]$, then $\mathrm{Im}\{\hat{h}_1(z)\} = 0$ there and (1) is satisfied. On the meniscus, $z = O(\delta)$, $\mathrm{Re}\{\hat{h}_s(z)\} = \chi(z)$, and $\mathrm{Re}\{h_s(z)\} = 0$, so

$$\begin{aligned}
\mathrm{Re}\{\hat{h}_1(z)\} &= \chi(z) + \mathrm{Re}\left\{\frac{2\hat{\lambda}_1}{\pi z} - \hat{\lambda}_1 \cot\left(\frac{\pi z}{2}\right) - \frac{\pi\hat{\lambda}_1}{6}z\right\} \\
&= \chi(z) + \mathrm{Re}\left\{\hat{\lambda}_1\frac{\pi^3}{360}z^3 + O(\hat{\lambda}_1\delta^5)\right\} = f(z) + O(\hat{\lambda}_1\delta^3) \\
&= \chi(z) + O(\delta^5).
\end{aligned}$$

Therefore (7) is satisfied to at least $O(\delta^4)$.

# 2 Symmetric channel with longitudinal ridges on both walls

In this section we present details analogous to those in the main paper, but for the case of a channel that is symmetric about its centreline, with longitudinal ridges on both the bottom and top walls. If a quantity differs from the corresponding quantity for the case of a smooth upper wall, it will be marked with a superscript "$(s)$", otherwise it can be assumed to be the same quantity as defined in the paper. The no-slip condition at $y^* = H^*$ is replaced by a symmetry condition, $\partial w^*/\partial y^* = 0$ at $y^* = H^*/2$. Scaling lengths still with $H^*$, the nondimensional problem is

$$\nabla^2 w^{(s)} = -2, \tag{32}$$

$$\frac{\partial w^{(s)}}{\partial y} = 0, \qquad \text{on } y = 1/2,\ x \in [-\epsilon, \epsilon] \tag{33}$$

$$w^{(s)} = 0, \qquad \text{on } y = 0,\ x \notin [-\epsilon\delta, \epsilon\delta], \tag{34}$$

$$\mathbf{n} \cdot \nabla w^{(s)} = 0, \qquad \text{on the meniscus } S, \tag{35}$$

$$\frac{\partial w^{(s)}}{\partial x} = 0, \qquad \text{on } x = \pm\epsilon,\ y \in [0, 1/2], \tag{36}$$

which is now only for half the channel, $y \leq 1/2$. Thus the quantity $Q^{(s)}$ denotes the flow rate per unit width through the bottom half of the channel.

For $\epsilon = l^*/H^* \ll 1$, the outer solution in the region $y = O(1)$ is

$$w^{(s)} = -y^2 + y + \epsilon\hat{\lambda}^{(s)}(\epsilon), \tag{37}$$

and if the solution in the inner region $(x, y) = (\epsilon X, \epsilon Y) = O(\epsilon)$ is $W^{(s)}$, then $W^{(s)}$ satisfies the matching condition

$$W^{(s)} \sim -\epsilon^2 Y^2 + \epsilon Y + \epsilon\hat{\lambda}^{(s)}(\epsilon), \qquad Y \to \infty. \tag{38}$$

Making the transformation $W^{(s)} = -\epsilon^2 Y^2 + \epsilon\widehat{W}^{(s)}$, the problem for $\widehat{W}^{(s)}$ on a semi-infinite strip is

$$\frac{\partial^2 \widehat{W}^{(s)}}{\partial X^2} + \frac{\partial^2 \widehat{W}^{(s)}}{\partial Y^2} = 0, \tag{39}$$

$$\widehat{W}^{(s)} = 0, \qquad \text{on } Y = 0,\ X \notin [-\delta, \delta] \tag{40}$$

$$\mathbf{n} \cdot \nabla_{XY}\widehat{W}^{(s)} = \mathbf{n} \cdot \nabla_{XY}(\epsilon Y^2), \qquad \text{on the meniscus } S, \tag{41}$$

$$\widehat{W}^{(s)} \sim Y + \hat{\lambda}^{(s)}(\epsilon), \qquad \text{as } Y \to \infty, \tag{42}$$

along with symmetry conditions $\partial\widehat{W}^{(s)}/\partial X = 0$ at $X = \pm 1$. This inner problem is the same as that for the case of a smooth upper wall but with the factor of $[1 + \epsilon\hat{\lambda}^{(s)}(\epsilon)]$ not appearing in the meniscus condition, (41). Consequently, the solution is slightly simpler as it does not implicitly depend on $\hat{\lambda}^{(s)}(\epsilon)$. The complex potential, $h_s^{(s)}(z)$, for a single meniscus occupying $X \in [-\delta, \delta]$ is therefore given by the Poisson integral formula (12), but without the factor of $[1 + \epsilon\hat{\lambda}^{(s)}(\epsilon)]$ that appears in $\chi(z)$, which is given by (7). Application of the reciprocal result gives

$$\hat{\lambda}^{(s)}(\epsilon) = \lambda - \epsilon \int_S YV \,\mathrm{d}X, \tag{43}$$

and substituting the approximations for $\lambda$ and $V$ for $\delta \ll 1$ give the approximations

$$\hat{\lambda}_0^{(s)}(\epsilon) = \lambda_0 - \epsilon\delta^3 I(\theta), \tag{44}$$

$$\hat{\lambda}_1^{(s)}(\epsilon) = \lambda_1 - \left(1 + \frac{\pi}{6}\lambda_1\right)\epsilon\delta^3 I(\theta). \tag{45}$$

The complex potential $\hat{h}_1^{(s)}$ is identical to (25) but with $\hat{h}_s(z)$ and $\hat{\lambda}_1(\epsilon)$ replaced with $\hat{h}_s^{(s)}(z)$ and $\hat{\lambda}_1^{(s)}(\epsilon)$.

To calculate $Q^{(s)}$, applying Green's second identity over the new domain ($y \leq 1/2$) gives (with $n$ the inward normal)

$$2\epsilon Q^{(s)} = -\int_{y\leq 1/2} y^2 \mathrm{d}A + 2\epsilon\left[\frac{1}{8} + \frac{1}{2}\epsilon\hat{\lambda}^{(s)}\right] + \int_S y^3 \frac{\partial y}{\partial n}\mathrm{d}s - \epsilon\int_S \widehat{W}^{(s)} y \frac{\partial y}{\partial n}\mathrm{d}s,$$

or, after substituting $\widehat{W}^{(s)} \sim \mathrm{Im}\{\hat{h}_s^{(s)}(z) + \frac{\pi}{6}\hat{\lambda}_1^{(s)} h_s(z)\}$,

$$Q^{(s)} = \frac{1}{12} + \frac{1}{2}\epsilon\hat{\lambda}^{(s)} + Q'^{(s)}, \tag{46}$$

with

$$Q'^{(s)} = -\frac{1}{2}\epsilon^2\delta^3(1 + \frac{\pi}{6}\hat{\lambda}_1^{(s)})I(\theta) + +\frac{1}{2}\epsilon^3\delta^4\left[F(\theta) - G(\theta)\right] + O(\delta^7). \tag{47}$$

The appropriate effective Navier slip profile is one that has the same slip length $\beta^{(s)}$ on both walls, i.e., $w_{NS}^{(s)} = \pm\beta^{(s)}\mathrm{d}w_{NS}^{(s)}/\mathrm{d}y$ on $y = 0, 1$, respectively, giving

$$w_{NS}^{(s)} = -y^2 + y + \beta^{(s)}. \tag{48}$$

Equating the flow rate (for $y \le 1/2$) per unit width with $Q^{(s)}$ results in

$$\beta^{(s)} = \epsilon\hat{\lambda}^{(s)} + 2Q'^{(s)}, \tag{49}$$

or, after substituting (45) and (47), we arrive at:

$$\beta^{(s)} = \epsilon\lambda_1 - \epsilon^2\delta^3 I\left(1 + \frac{\pi}{6}\lambda_1\right)\left(2 - \frac{\pi}{6}\epsilon\delta^3 I\right) + \epsilon^3\delta^4(F - G), \tag{50}$$

given as (1.5) in the paper.

## 2.1 Verification against previous work: small meniscus curvature formulae

The case of longitudinal ridges on both channel walls and has already been considered by Kirk *et al.* [3] for small meniscus curvature or protrusion, $|\theta| \ll 1$, and arbitrary $\epsilon$, $\delta$. In particular, an analytic expression for the slip length was found to all algebraic orders in $\epsilon \ll 1$,

$$\begin{aligned}\frac{\beta^{(s)}}{\epsilon} =& \frac{2}{\pi}\log\left[\sec\left(\frac{\pi\delta}{2}\right)\right] - \frac{\theta}{2\delta}\left(-\delta^3\int_0^1 \frac{[1-\cos(\delta\pi s)](1-s^2)\,\mathrm{d}s}{\cos(\delta\pi s) - \cos(\delta\pi)}\right.\\ &\left. + 4\epsilon\delta^4\sqrt{2}\int_0^1 \frac{s(1-s^2/3)\sin(\delta\pi s/2)\,\mathrm{d}s}{\sqrt{\cos(\delta\pi s) - \cos(\delta\pi)}}\right) + O(\theta^2).\end{aligned} \tag{51}$$

Expanding this solution for $\delta \ll 1$ should agree with (50) expanded for $|\theta| \ll 1$. Each term in (51) has expansion for $\delta \ll 1$,

$$\frac{2}{\pi}\log\left[\sec\left(\frac{\pi\delta}{2}\right)\right] = \frac{\pi\delta^2}{4} + \frac{\pi^3\delta^4}{96} + O(\delta^6),$$

$$\delta^3\int_0^1 \frac{[1-\cos(\delta\pi s)](1-s^2)\,\mathrm{d}s}{\cos(\delta\pi s) - \cos(\delta\pi)} = \frac{\delta^3}{3} + \frac{\pi^2\delta^5}{36} + O(\delta^7),$$

$$\delta^4\int_0^1 \frac{s(1-s^2/3)\sin(\delta\pi s/2)\,\mathrm{d}s}{\sqrt{\cos(\delta\pi s) - \cos(\delta\pi)}} = \frac{3\sqrt{2}\pi\delta^4}{16} + O(\delta^6),$$

giving

$$\frac{\beta^{(s)}}{\epsilon} = \left(\frac{\pi\delta^2}{4} + \frac{\pi^3\delta^4}{96} + O(\delta^6)\right) + \theta\left[\left(\frac{\delta^3}{6} + \frac{\pi^2\delta^5}{72} + O(\delta^7)\right) - \epsilon\left(\frac{3\pi\delta^4}{4} + O(\delta^6)\right)\right] + O(\theta^2). \tag{52}$$

Now, we expand our formula (50) for $|\theta| \ll 1$ up to $O(\theta)$. It can be shown that $F = O(\theta^3)$, $G = O(\theta^2)$, $I = \frac{3}{16}\pi\theta + O(\theta^2)$ for $|\theta| \ll 1$, and $\lambda_1$ expanded for $|\theta|, \delta \ll 1$ is

$$\lambda_1 = \left(\frac{\pi\delta^2}{4} + \frac{\pi^3\delta^4}{96} + O(\delta^6)\right) + \theta\left(\frac{\delta^3}{6} + \frac{\pi^2\delta^5}{72} + O(\delta^7)\right) + O(\theta^2). \tag{53}$$

After substituting these into (50), it reduces exactly to the expression (52) up to the orders given, as expected. Note that they agree up to at least fifth order in $\delta$.

# References


[1] D. G. Crowdy, *Slip length for longitudinal shear flow over a dilute periodic mattress of protruding bubbles*, Phys. Fluids **22** (2010), no. 12, 121703.

[2] ———, *Analytical formulae for longitudinal slip lengths over unidirectional superhydrophobic surfaces with curved menisci*, J. Fluid Mech. **791** (2016), no. R7.

[3] T. L. Kirk, M. Hodes, and D. T. Papageorgiou, *Nusselt numbers for Poiseuille flow over isoflux parallel ridges accounting for meniscus curvature*, J. Fluid Mech. **811** (2017), 315–349.

[4] Z. Nehari, *Conformal mapping*, 1975 reprint ed., Dover, 1952.
